# Supplementary material for: Efficient QAM Signal Detector for Massive MIMO Systems via PS-ADMM Approach
Source: arXiv:2104.08064 source file (2021-12-11)
Supplement: Supplementary file 1 [file PS-ADMM-Supplementary.pdf]

# Efficient QAM Signal Detector for Massive MIMO Systems via PS-ADMM Approach

## (Supplementary Material)

Quan Zhang, Jiangtao Wang, Yongchao Wang, *Senior Member, IEEE*

In this section, we firstly briefly present the proposed penalty-sharing problem and the corresponding DPS-ADMM algorithm in Section 1, followed by the convergence analysis and iteration complexity analysis about the DPS-ADMM algorithms for the penalty-sharing program problems in Section 2 and Section 3, respectively.

### 1. DPS-ADMM Algorithm for the penalty-sharing Problem

We approximate maximum-likelihood detection problem to formulate the following non-convex penalty-sharing problem

$$\begin{aligned} \min_{\mathbf{x}_q} \quad & \frac{1}{2} \|\mathbf{r} - \mathbf{H}(\sum_{q=1}^Q 2^{q-1} \mathbf{x}_q)\|_2^2 - \sum_{q=1}^Q \frac{\alpha_q}{2} \|\mathbf{x}_q\|_2^2, \\ \text{s.t.} \quad & \mathbf{x}_q \in \tilde{\mathbb{X}}_q^U, \quad q = 1, \dots, Q, \end{aligned} \tag{1}$$

where penalty parameters  $\alpha_q \geq 0$  and  $\tilde{\mathbb{X}}_q = \{x_{qR} + jx_{qI} | x_{qR}, x_{qI} \in [1, -1]\}$ .

We develop an efficient ADMM algorithm, named DPS-ADMM, to solve the model (1) via distributed approach. We introduce a auxiliary variable  $\mathbf{z}_q \in \mathbb{C}^U$  to replace  $2^{q-1} \mathbf{x}_q$ , the model

(1) be transformed equivalently to a sharing problem as follows

$$\begin{aligned}
\min_{\mathbf{z}_q, \mathbf{x}_q} \quad & \frac{1}{2} \|\mathbf{r} - \mathbf{H} \sum_{q=1}^Q \mathbf{z}_q\|_2^2 - \sum_{q=1}^Q \frac{\alpha_q}{2} \|\mathbf{x}_q\|_2^2, \\
\text{s.t.} \quad & \mathbf{z}_q = 2^{q-1} \mathbf{x}_q, \\
& \mathbf{x}_q \in \tilde{\mathbb{X}}_q^U, q = 1, \dots, Q.
\end{aligned} \tag{2}$$

The proposed DPS-ADMM algorithm for the model (2) can be derived directly from the augmented Lagrangian

$$\begin{aligned}
L_\rho(\{\mathbf{x}_q, \mathbf{z}_q, \mathbf{y}_q\}_{q=1}^Q) = & \frac{1}{2} \|\mathbf{r} - \mathbf{H} \sum_{q=1}^Q \mathbf{z}_q\|_2^2 - \sum_{q=1}^Q \frac{\alpha_q}{2} \|\mathbf{x}_q\|_2^2 \\
& + \sum_{q=1}^Q \text{Re} \langle 2^{q-1} \mathbf{x}_q - \mathbf{z}_q, \mathbf{y}_q \rangle + \sum_{q=1}^Q \frac{\rho}{2} \|2^{q-1} \mathbf{x}_q - \mathbf{z}_q\|_2^2,
\end{aligned} \tag{3}$$

where  $\mathbf{y}_q \in \mathbb{C}^U$  and  $\rho > 0$  are the Lagrangian multipliers and penalty parameter respectively.

The resulting DPS-ADMM algorithm is the following

$$\mathbf{x}_q^{k+1} = \arg \min_{\mathbf{x}_q \in \tilde{\mathbb{X}}_q^U} L_\rho(\mathbf{x}_q, \{\mathbf{z}_q^k, \mathbf{y}_q^k\}_{q=1}^Q), \tag{4a}$$

$$\mathbf{z}_q^{k+1} = \arg \min_{\mathbf{z}_q} L_\rho(\mathbf{z}_q, \{\mathbf{x}_q^{k+1}, \mathbf{y}_q^k\}_{q=1}^Q), \tag{4b}$$

$$\mathbf{y}_q^{k+1} = \mathbf{y}_q^k + \rho \left( 2^{q-1} \mathbf{x}_q^{k+1} - \mathbf{z}_q^{k+1} \right), \tag{4c}$$

where  $q = 1, \dots, Q$ ,  $k$  denotes iteration number.

## 2. Convergence Analysis

We have the following theorem to show convergence properties of the proposed DPS-ADMM algorithm.

*Theorem 1:* Assume  $4^{q-1} \rho > \alpha_q, q = 1, \dots, Q$  and  $\rho > \sqrt{2} \lambda_{\max}(\mathbf{H}^H \mathbf{H})$  are satisfied. Then,

sequence  $\{\{\mathbf{x}_q, \mathbf{z}_q, \mathbf{y}_q\}_{q=1}^Q\}$  generated by DPS-ADMM Algorithm is convergent, i.e.,

$$\begin{aligned} \lim_{k \rightarrow +\infty} \mathbf{x}_q^k &= \mathbf{x}_q^*, \quad \lim_{k \rightarrow +\infty} \mathbf{z}_q^k = \mathbf{z}_q^*, \quad \lim_{k \rightarrow +\infty} \mathbf{y}_q^k = \mathbf{y}_q^*, \\ \forall \mathbf{x}_q &\in \tilde{\mathbb{X}}_q^U, \quad q = 1, \dots, Q. \end{aligned} \quad (5)$$

Moreover,  $\{\mathbf{x}_q^*\}_{q=1}^Q$  is a stationary point of problem (1), i.e.,  $\forall \mathbf{x}_q \in \tilde{\mathbb{X}}_q^U, \quad q = 1, \dots, Q$ , which satisfies

$$\text{Re} \left\langle \nabla_{\mathbf{x}_q} \left( \frac{1}{2} \|\mathbf{r} - \mathbf{H}(\sum_{q=1}^Q 2^{q-1} \mathbf{x}_q^*)\|_2^2 - \sum_{q=1}^Q \frac{\alpha_q}{2} \|\mathbf{x}_q^*\|_2^2 \right), \mathbf{x}_q - \mathbf{x}_q^* \right\rangle \geq 0. \quad (6)$$

Theorem 1 indicates that the proposed DPS-ADMM algorithm is theoretically-guaranteed converged to some stationary point of the model (1) under some wild conditions. Here, we should note that these conditions are easily satisfied since the values of penalty parameters  $\rho$  and  $\{\alpha_q\}_{q=1}^Q$  can be set accordingly when the channel matrix  $\mathbf{H}$  is known. The key idea of proving Theorem 1 is to find out that the potential function  $L_\rho(\{\mathbf{x}_q, \mathbf{z}_q, \mathbf{y}_q\}_{q=1}^Q)$  *decreases sufficiently* in every DPS-ADMM iteration and is lower-bounded. To reach this goal, we first prove several related lemmas and then provide detailed proof of Theorem 1. For simplicity of notation, we use  $\ell(\mathbf{x})$  to denote  $\frac{1}{2} \|\mathbf{r} - \mathbf{H}\mathbf{x}\|_2^2$  in the rest of this paper.

Before proving convergence of the proposed PS-ADMM algorithm, we give several lemmas and their proofs as follows.

*Lemma 1:* For Algorithm 1, the following inequality holds

$$\|\mathbf{y}_q^{k+1} - \mathbf{y}_q^k\|_2^2 \leq \lambda_{\max}^2(\mathbf{H}^H \mathbf{H}) \|\mathbf{z}_q^{k+1} - \mathbf{z}_q^k\|_2^2, \quad (7)$$

where  $\lambda_{\max}(\cdot)$  denotes the maximum eigenvalues of a matrix.

*Proof:* Since  $\mathbf{z}_q^{k+1}$  is a minimizer of problem (4b), it should satisfy the following optimality condition [1]

$$\nabla_{\mathbf{z}_q} \ell(\mathbf{z}_q^{k+1}) - \mathbf{y}_q^k - \rho \left( \sum_{q=1}^Q 2^{q-1} \mathbf{x}_q^{k+1} - \mathbf{z}_q^{k+1} \right) = 0. \quad (8)$$

Plugging  $\mathbf{y}_q^{k+1}$  in (4c) into the above equation, we obtain

$$\mathbf{y}_q^{k+1} = \nabla_{\mathbf{z}_q} \ell(\mathbf{z}_q^{k+1}). \quad (9)$$

According to Lagrange's mean value theorem, since  $\ell(\mathbf{z}_q)$  is continuous and differentiable, there exists some point  $\bar{\mathbf{z}}_q$  between  $\mathbf{z}_q^k$  and  $\mathbf{z}_q^{k+1}$  which satisfies

$$\frac{\nabla_{\mathbf{z}_q} \ell(\mathbf{z}_q^{k+1}) - \nabla_{\mathbf{z}_q} \ell(\mathbf{z}_q^k)}{\mathbf{z}_q^{k+1} - \mathbf{z}_q^k} = \nabla_{\bar{\mathbf{z}}_q}^2 \ell(\mathbf{z}_q). \quad (10)$$

Moreover, since  $\nabla_{\bar{\mathbf{z}}_q}^2 \ell(\mathbf{z}_q) = \mathbf{H}^H \mathbf{H} \preceq \lambda_{\max}(\mathbf{H}^H \mathbf{H}) \mathbf{I}$ , we have

$$\|\nabla_{\mathbf{z}_q} \ell(\mathbf{z}_q^{k+1}) - \nabla_{\mathbf{z}_q} \ell(\mathbf{z}_q^k)\|_2^2 \leq \lambda_{\max}^2(\mathbf{H}^H \mathbf{H}) \|\mathbf{z}_q^{k+1} - \mathbf{z}_q^k\|_2^2. \quad (11)$$

From (11), we can see that  $\nabla_{\mathbf{z}_q} \ell(\mathbf{z}_q)$  is Lipschitz continuous with constant  $\lambda_{\max}(\mathbf{H}^H \mathbf{H})$ . Plugging (9) into LHS of equation (11), we can obtain

$$\|\mathbf{y}_q^{k+1} - \mathbf{y}_q^k\|_2^2 = \|\nabla_{\mathbf{z}_q} \ell(\mathbf{z}_q^{k+1}) - \nabla_{\mathbf{z}_q} \ell(\mathbf{z}_q^k)\|_2^2 \leq \lambda_{\max}^2(\mathbf{H}^H \mathbf{H}) \|\mathbf{z}_q^{k+1} - \mathbf{z}_q^k\|_2^2.$$

This completes the proof. ■

*Lemma 2:* Let  $\alpha_q$  and  $\rho$  satisfy  $4^{q-1}\rho > \alpha_q$ ,  $\forall q \in \{1, \dots, Q\}$ . Then, for Algorithm 1, we have the following inequality

$$\begin{aligned} & L_\rho \left( \{\mathbf{x}_q^{k+1}, \mathbf{z}_q^{k+1}, \mathbf{y}_q^{k+1}\}_{q=1}^Q \right) - L_\rho \left( \{\mathbf{x}_q^k, \mathbf{z}_q^k, \mathbf{y}_q^k\}_{q=1}^Q \right) \\ & \leq \sum_{q=1}^Q \frac{\gamma_q(\rho)}{2} \|\mathbf{x}_q^{k+1} - \mathbf{x}_q^k\|_2^2 - \sum_{q=1}^Q \left( \frac{\gamma_0(\rho)}{2} - \frac{\lambda_{\max}^2(\mathbf{H}^H \mathbf{H})}{\rho} \right) \|\mathbf{z}_q^{k+1} - \mathbf{z}_q^k\|_2^2, \end{aligned} \quad (12)$$

where  $\gamma_q(\rho) = 4^{q-1}\rho - \alpha_q$  and  $\gamma_0(\rho) = \rho + \lambda_{\min}(\mathbf{H}^H \mathbf{H})$ ,  $\lambda_{\min}(\cdot)$  denotes the minimum eigenvalues of a matrix.

*Proof:* We split LHS of the inequality (12) into two terms

$$\begin{aligned}
& L_\rho(\{\mathbf{x}_q^{k+1}, \mathbf{z}_q^{k+1}, \mathbf{y}_q^{k+1}\}_{q=1}^Q) - L_\rho(\{\mathbf{x}_q^k, \mathbf{z}_q^k, \mathbf{y}_q^k\}_{q=1}^Q) \\
&= \underbrace{\left( L_\rho(\{\mathbf{x}_q^{k+1}, \mathbf{z}_q^{k+1}, \mathbf{y}_q^{k+1}\}_{q=1}^Q) - L_\rho(\{\mathbf{x}_q^{k+1}, \mathbf{z}_q^{k+1}, \mathbf{y}_q^k\}_{q=1}^Q) \right)}_{\text{term 1}} \\
&\quad + \underbrace{\left( L_\rho(\{\mathbf{x}_q^{k+1}, \mathbf{z}_q^{k+1}, \mathbf{y}_q^k\}_{q=1}^Q) - L_\rho(\{\mathbf{x}_q^k, \mathbf{z}_q^k, \mathbf{y}_q^k\}_{q=1}^Q) \right)}_{\text{term 2}}.
\end{aligned}$$

For the first term, we have the following derivations

$$\begin{aligned}
& L_\rho(\{\mathbf{x}_q^{k+1}, \mathbf{z}_q^{k+1}, \mathbf{y}_q^{k+1}\}_{q=1}^Q) - L_\rho(\{\mathbf{x}_q^{k+1}, \mathbf{z}_q^{k+1}, \mathbf{y}_q^k\}_{q=1}^Q) \\
&= \sum_{q=1}^Q \left( \text{Re} \langle 2^{q-1} \mathbf{x}_q^{k+1} - \mathbf{z}_q^{k+1}, \mathbf{y}_q^{k+1} \rangle - \text{Re} \langle 2^{q-1} \mathbf{x}_q^{k+1} - \mathbf{z}_q^{k+1}, \mathbf{y}_q^k \rangle \right) \\
&= \sum_{q=1}^Q \text{Re} \langle 2^{q-1} \mathbf{x}_q^{k+1} - \mathbf{z}_q^{k+1}, \mathbf{y}_q^{k+1} - \mathbf{y}_q^k \rangle \\
&\stackrel{(a)}{=} \frac{1}{\rho} \sum_{q=1}^Q \|\mathbf{y}_q^{k+1} - \mathbf{y}_q^k\|_2^2 \\
&\stackrel{(b)}{\leq} \frac{\lambda_{\max}^2(\mathbf{H}^H \mathbf{H})}{\rho} \sum_{q=1}^Q \|\mathbf{z}_q^{k+1} - \mathbf{z}_q^k\|_2^2,
\end{aligned} \tag{13}$$

where “ $\stackrel{(a)}{=}$ ” and “ $\stackrel{(b)}{\leq}$ ” comes from (4c) and (7) respectively.

For the second term, we have the following derivations

$$\begin{aligned}
& L_\rho(\{\mathbf{x}_q^{k+1}, \mathbf{z}_q^{k+1}, \mathbf{y}_q^k\}_{q=1}^Q) - L_\rho(\{\mathbf{x}_q^k, \mathbf{z}_q^k, \mathbf{y}_q^k\}_{q=1}^Q) \\
&= L_\rho(\{\mathbf{x}_q^{k+1}, \mathbf{z}_q^k, \mathbf{y}_q^k\}_{q=1}^Q) - L_\rho(\{\mathbf{x}_q^k, \mathbf{z}_q^k, \mathbf{y}_q^k\}_{q=1}^Q) \\
&+ L_\rho(\{\mathbf{x}_q^{k+1}, \mathbf{z}_q^{k+1}, \mathbf{y}_q^k\}_{q=1}^Q) - L_\rho(\{\mathbf{x}_q^{k+1}, \mathbf{z}_q^k, \mathbf{y}_q^k\}_{q=1}^Q) \\
&\leq \sum_{q=1}^Q \left( \text{Re} \left\langle \nabla_{\mathbf{x}_q} L_\rho(\mathbf{x}_1^{k+1}, \dots, \mathbf{x}_{q-1}^{k+1}, \mathbf{x}_q^k, \mathbf{x}_{q+1}^k, \dots, \mathbf{x}_Q^k, \{\mathbf{z}_q^{k+1}, \mathbf{y}_q^k\}_{q=1}^Q), \mathbf{x}_q^{k+1} - \mathbf{x}_q^k \right\rangle \right. \\
&\quad \left. - \frac{4^{q-1}\rho - \alpha_q}{2} \|\mathbf{x}_q^{k+1} - \mathbf{x}_q^k\|_2^2 \right) \\
&+ \sum_{q=1}^Q \left( \text{Re} \left\langle \nabla_{\mathbf{z}_q} L_\rho(\mathbf{z}_1^{k+1}, \dots, \mathbf{z}_{q-1}^{k+1}, \mathbf{z}_q^k, \mathbf{z}_{q+1}^k, \dots, \mathbf{z}_Q^k, \{\mathbf{x}_q^{k+1}, \mathbf{y}_q^k\}_{q=1}^Q), \mathbf{z}_q^{k+1} - \mathbf{z}_q^k \right\rangle \right. \\
&\quad \left. - \frac{\rho + \lambda_{\min}(\mathbf{H}^H \mathbf{H})}{2} \|\mathbf{z}_q^{k+1} - \mathbf{z}_q^k\|_2^2 \right) \\
&\leq \sum_{q=1}^Q \frac{\alpha_q - 4^{q-1}\rho}{2} \|\mathbf{x}_q^{k+1} - \mathbf{x}_q^k\|_2^2 - \sum_{q=1}^Q \frac{\rho + \lambda_{\min}(\mathbf{H}^H \mathbf{H})}{2} \|\mathbf{z}_q^{k+1} - \mathbf{z}_q^k\|_2^2,
\end{aligned} \tag{14}$$

where the first inequality holds since the corresponding augmented Lagrangian functions are strongly convex [2] and the second inequality holds since  $\mathbf{x}_q^{k+1}$  and  $\mathbf{z}_q^{k+1}$  are minimizers of the problems (4a) and (4b), i.e.,

$$\begin{aligned}
& \left\langle \nabla_{\mathbf{x}_q} L_\rho(\mathbf{x}_q^{k+1}, \mathbf{x}_1^{k+1}, \dots, \mathbf{x}_{q-1}^{k+1}, \mathbf{x}_{q+1}^k, \dots, \mathbf{x}_Q^k, \{\mathbf{z}_q^{k+1}, \mathbf{y}_q^k\}_{q=1}^Q), \mathbf{x}_q^k - \mathbf{x}_q^{k+1} \right\rangle \geq 0 \\
& \nabla_{\mathbf{z}_q} L_\rho(\mathbf{z}_q^{k+1}, \mathbf{z}_1^{k+1}, \dots, \mathbf{z}_{q-1}^{k+1}, \mathbf{z}_{q+1}^k, \dots, \mathbf{z}_Q^k, \{\mathbf{x}_q^{k+1}, \mathbf{y}_q^k\}_{q=1}^Q) = 0.
\end{aligned}$$

Adding both sides of inequalities (13) and (14) and letting  $\gamma_q(\rho) = 4^{q-1}\rho - \alpha_q$  and  $\gamma_0(\rho) = \rho + \lambda_{\min}(\mathbf{H}^H \mathbf{H})$ , we can obtain

$$\begin{aligned}
& L_\rho(\{\mathbf{x}_q^{k+1}, \mathbf{z}_q^{k+1}, \mathbf{y}_q^{k+1}\}_{q=1}^Q) - L_\rho(\{\mathbf{x}_q^k, \mathbf{z}_q^k, \mathbf{y}_q^k\}_{q=1}^Q) \\
&\leq \sum_{q=1}^Q -\frac{\gamma_q(\rho)}{2} \|\mathbf{x}_q^{k+1} - \mathbf{x}_q^k\|_2^2 - \sum_{q=1}^Q \left( \frac{\gamma_0(\rho)}{2} - \frac{\lambda_{\max}^2(\mathbf{H}^H \mathbf{H})}{\rho} \right) \|\mathbf{z}_q^{k+1} - \mathbf{z}_q^k\|_2^2,
\end{aligned}$$

which completes the proof. ■

*Lemma 3:* Let  $\alpha_q, \forall q \in \{1, \dots, Q\}$ , and  $\rho$  satisfy  $4^{q-1}\rho > \alpha_q$  and  $\rho > \sqrt{2}\lambda_{\max}(\mathbf{H}^H\mathbf{H})$ . Assume tuples  $\{\{\mathbf{x}_q^k, \mathbf{z}_q^k, \mathbf{y}_q^k\}_{q=1}^Q\}$  is generated by Algorithm 1, then  $L_\rho(\{\mathbf{x}_q^k, \mathbf{z}_q^k, \mathbf{y}_q^k\}_{q=1}^Q)$  is lower bounded as follows

$$L_\rho(\{\mathbf{x}_q^k, \mathbf{z}_q^k, \mathbf{y}_q^k\}_{q=1}^Q) \geq \ell(2^{q-1}\mathbf{x}_q^k) - \sum_{q=1}^Q \frac{\alpha_q}{2} \|\mathbf{x}_q^k\|_2^2. \quad (15)$$

*Proof:* Plugging (9) into (3), we obtain

$$\begin{aligned} L_\rho(\{\mathbf{x}_q^k, \mathbf{z}_q^k, \mathbf{y}_q^k\}_{q=1}^Q) &= \ell(\mathbf{z}_q^k) - \sum_{q=1}^Q \frac{\alpha_q}{2} \|\mathbf{x}_q^k\|_2^2 \\ &\quad + \text{Re} \left\langle 2^{q-1}\mathbf{x}_q^k - \mathbf{z}_q^k, \nabla_{\mathbf{z}_q} \ell(\mathbf{z}_q^k) \right\rangle + \frac{\rho}{2} \left\| 2^{q-1}\mathbf{x}_q^k - \mathbf{z}_q^k \right\|_2^2. \end{aligned} \quad (16)$$

Since we show that gradient  $\|\nabla_{\mathbf{z}_q} \ell(\mathbf{z}_q)\|_2$  is Lipschitz continuous in Lemma 1 and  $\|\nabla_{\mathbf{z}_q}^2 \ell(\mathbf{z}_q)\|_2 \leq \lambda_{\max}(\mathbf{H}^H\mathbf{H})$ , according to the Decent Lemma [3], we can obtain

$$\ell(2^{q-1}\mathbf{x}_q^k) \leq \ell(\mathbf{z}_q^k) + \text{Re} \left\langle \nabla_{\mathbf{z}_q} \ell(\mathbf{z}_q^k), 2^{q-1}\mathbf{x}_q^k - \mathbf{z}_q^k \right\rangle + \frac{\lambda_{\max}(\mathbf{H}^H\mathbf{H})}{2} \left\| 2^{q-1}\mathbf{x}_q^k - \mathbf{z}_q^k \right\|_2^2,$$

which can be further derived to the following inequality

$$\ell(\mathbf{z}_q^k) + \text{Re} \left\langle 2^{q-1}\mathbf{x}_q^k - \mathbf{z}_q^k, \nabla_{\mathbf{z}_q} \ell(\mathbf{z}_q^k) \right\rangle \geq \ell(2^{q-1}\mathbf{x}_q^k) - \frac{\lambda_{\max}(\mathbf{H}^H\mathbf{H})}{2} \left\| 2^{q-1}\mathbf{x}_q^k - \mathbf{z}_q^k \right\|_2^2. \quad (17)$$

Plugging (17) into (16), we can get

$$L_\rho(\{\mathbf{x}_q^k, \mathbf{z}_q^k, \mathbf{y}_q^k\}_{q=1}^Q) \geq \ell(2^{q-1}\mathbf{x}_q^k) - \sum_{q=1}^Q \frac{\alpha_q}{2} \|\mathbf{x}_q^k\|_2^2 + \frac{\rho - \lambda_{\max}(\mathbf{H}^H\mathbf{H})}{2} \left\| \mathbf{z}_q^k - 2^{q-1}\mathbf{x}_q^k \right\|_2^2. \quad (18)$$

Since  $\ell(2^{q-1}\mathbf{x}_q^k) - \sum_{q=1}^Q \frac{\alpha_q}{2} \|\mathbf{x}_q^k\|_2^2$  is bounded over  $\mathbf{x}_{qR}, \mathbf{x}_{qI} \in [-1 \ 1]^U$ , as well as the fact that  $\rho - \lambda_{\max}(\mathbf{H}^H\mathbf{H}) > 0$  comes from  $\rho > \sqrt{2}\lambda_{\max}(\mathbf{H}^H\mathbf{H})$ . Using these two cases leads to the desired result that  $L_\rho(\{\mathbf{x}_q^k, \mathbf{z}_q^k, \mathbf{y}_q^k\}_{q=1}^Q)$  is lower bounded and Lemma 3 has been proved. ■

According to Lemma 2, summing both sides of the inequality (12) when  $k = 1, 2, \dots, +\infty$ , we can obtain

$$\begin{aligned}
& L_\rho \left( \{\mathbf{x}_q^1, \mathbf{z}_q^1, \mathbf{y}_q^1\}_{q=1}^Q \right) - \lim_{k \rightarrow +\infty} L_\rho \left( \{\mathbf{x}_q^k, \mathbf{z}_q^k, \mathbf{y}_q^k\}_{q=1}^Q \right) \\
& \geq \sum_{k=1}^{+\infty} \sum_{q=1}^Q \frac{\gamma_q(\rho)}{2} \|\mathbf{x}_q^{k+1} - \mathbf{x}_q^k\|_2^2 \\
& + \sum_{k=1}^{+\infty} \sum_{q=1}^Q \left( \frac{\gamma_0(\rho)}{2} - \frac{\lambda_{\max}^2(\mathbf{H}^H \mathbf{H})}{\rho} \right) \|\mathbf{z}_q^{k+1} - \mathbf{z}_q^k\|_2^2.
\end{aligned} \tag{19}$$

From Lemma 3, one can see that  $\lim_{k \rightarrow +\infty} L_\rho \left( \{\mathbf{x}_q^k, \mathbf{z}_q^k, \mathbf{y}_q^k\}_{q=1}^Q \right) > -\infty$ . Moreover, since  $\frac{\gamma_0(\rho)}{2} - \frac{\lambda_{\max}^2(\mathbf{H}^H \mathbf{H})}{\rho} \geq 0$ , we can obtain

$$\lim_{k \rightarrow +\infty} \|\mathbf{z}_q^{k+1} - \mathbf{z}_q^k\|_2 = 0, \tag{20a}$$

$$\lim_{k \rightarrow +\infty} \|\mathbf{x}_q^{k+1} - \mathbf{x}_q^k\|_2 = 0, \quad q \in \{1, \dots, Q\}. \tag{20b}$$

Plugging (20a) into RHS of equation (7), we get

$$\lim_{k \rightarrow +\infty} \|\mathbf{y}_q^{k+1} - \mathbf{y}_q^k\|_2 = 0. \tag{21}$$

Plugging (21) into (4c), we get

$$\lim_{k \rightarrow +\infty} \|2^{q-1} \mathbf{x}_q^{k+1} - \mathbf{z}_q^{k+1}\|_2 = 0. \tag{22}$$

Since  $\mathbf{x}_{qR}, \mathbf{x}_{qI} \in [-1 \ 1]^U$ , we can obtain the following convergence results from (20b).

$$\lim_{k \rightarrow +\infty} \mathbf{x}_q^k = \mathbf{x}_q^*, \quad \forall q = 1, 2, \dots, Q. \tag{23}$$

Plugging (23) into (22), we can see

$$\lim_{k \rightarrow +\infty} \mathbf{z}_q^k = \mathbf{z}_q^* = 2^{q-1} \mathbf{x}_q^*. \tag{24}$$

From (9), we can derive

$$\lim_{k \rightarrow +\infty} \mathbf{y}_q^k = \lim_{k \rightarrow +\infty} \nabla_{\mathbf{z}_q} \ell(\mathbf{z}_q^k). \tag{25}$$



Since  $\|\nabla_{\mathbf{z}_q} \ell(\mathbf{z}_q^{k+1}) - \nabla_{\mathbf{z}_q} \ell(\mathbf{z}_q^k)\|_2^2 \leq \lambda_{\max}^2(\mathbf{H}^H \mathbf{H}) \|\mathbf{z}_q^{k+1} - \mathbf{z}_q^k\|_2^2$  and  $\mathbf{z}_q^k$  is bounded, we can conclude that all the elements in  $\nabla_{\mathbf{z}_q} \ell(\mathbf{z}_q)$  are also bounded. Therefore, equation (21) indicates

$$\lim_{k \rightarrow +\infty} \mathbf{y}_q^k = \mathbf{y}_q^*. \quad (26)$$

Then, we prove  $\{\mathbf{x}_q^*\}_{q=1}^Q$  is a stationary point of problem (1).

Since  $\{\mathbf{x}_q^{k+1}\}_{q=1}^Q = \arg \min_{\mathbf{x}_q \in \tilde{\mathbb{X}}_q^U} L_\rho(\{\mathbf{x}_q, \mathbf{z}_q^k, \mathbf{y}_q^k\}_{q=1}^Q)$  in (4a), and  $L_\rho(\{\mathbf{x}_q, \mathbf{z}_q^k, \mathbf{y}_q^k\}_{q=1}^Q)$  is strongly convex w.r.t.  $\mathbf{x}_q$ , we have the following optimality conditions.

$$\begin{aligned} & \text{Re} \left\langle \nabla_{\mathbf{x}_q} \left( \ell(\mathbf{z}_q^k) - \sum_{q=1}^Q \frac{\alpha_q}{2} \|\mathbf{x}_q^{k+1}\|_2^2 \right. \right. \\ & \left. \left. + \sum_{q=1}^Q \left\langle 2^{q-1} \mathbf{x}_q^{k+1} - \mathbf{z}_q^k, \mathbf{y}_q^k \right\rangle + \sum_{q=1}^Q \frac{\rho}{2} \|2^{q-1} \mathbf{x}_q^{k+1} - \mathbf{z}_q^k\|_2^2 \right), \mathbf{x}_q - \mathbf{x}_q^{k+1} \right\rangle \geq 0, \\ & \forall \mathbf{x}_q \in \tilde{\mathbb{X}}_q^U, q = 1, 2, \dots, Q. \end{aligned} \quad (27)$$

When  $k \rightarrow +\infty$ , plugging convergence results (23) and (24) into (27), it can be simplified as

$$\begin{aligned} & \text{Re} \left\langle \nabla_{\mathbf{x}_q} \left( \ell \left( \sum_{q=1}^Q 2^{q-1} \mathbf{x}_q^* \right) - \sum_{q=1}^Q \frac{\alpha_q}{2} \|\mathbf{x}_q^*\|_2^2 \right), \mathbf{x}_q - \mathbf{x}_q^* \right\rangle \geq 0, \\ & \forall \mathbf{x}_q \in \tilde{\mathbb{X}}_q^U, q = 1, 2, \dots, Q. \end{aligned}$$

which completes the proof. ■

### 3. Iteration Complexity Analysis

We use the following residual

$$\sum_{q=1}^Q \left( \|\mathbf{x}_q^{k+1} - \mathbf{x}_q^k\|_2^2 + \|\mathbf{z}_q^{k+1} - \mathbf{z}_q^k\|_2^2 \right) \quad (28)$$

to measure the convergence progress of the DPS-ADMM algorithm since it converges to zero as  $k \rightarrow +\infty$ . Then, we have Theorem 2 about its convergence progress, in which the "upper bound" of the "minimum" iteration gives an upper bound on the computational complexity of

the proposed DPS-ADMM algorithm in Section 1.

*Theorem 2:* Let  $t$  be the minimum iteration index such that the residual in (28) is less than  $\epsilon$ , where  $\epsilon$  is the desired precise parameter for the solution. Then, we have the following iteration complexity result

$$t \leq \frac{1}{C\epsilon} \left( L_\rho(\{\mathbf{x}_q^1, \mathbf{z}_q^1, \mathbf{y}_q^1\}_{q=1}^Q) - \left( \ell(\mathbf{z}_q^*) - \sum_{q=1}^Q \frac{\alpha_q}{2} \|\mathbf{x}_q^*\|_2^2 \right) \right),$$

where the constant

$$C = \min \left\{ \left\{ \frac{\gamma_q(\rho)}{2} \right\}_{q=1}^Q, \left( \frac{\gamma_0(\rho)}{2} - \frac{\lambda_{\max}^2(\mathbf{H}^H \mathbf{H})}{\rho} \right) \right\},$$

and  $\gamma_q(\rho) = 4^{q-1}\rho - \alpha_q$ ,  $\gamma_0(\rho) = \rho + \lambda_{\min}(\mathbf{H}^H \mathbf{H})$ .

*Proof:* To be clear, here we rewrite (12) as

$$\begin{aligned} & L_\rho \left( \{\mathbf{x}_q^k, \mathbf{z}_q^k, \mathbf{y}_q^k\}_{q=1}^Q \right) - L_\rho \left( \{\mathbf{x}_q^{k+1}, \mathbf{z}_q^{k+1}, \mathbf{y}_q^{k+1}\}_{q=1}^Q \right) \\ & \geq \sum_{q=1}^Q \frac{\gamma_q(\rho)}{2} \|\mathbf{x}_q^{k+1} - \mathbf{x}_q^k\|_2^2 + \sum_{q=1}^Q \left( \frac{\gamma(\rho)}{2} - \frac{\lambda_{\max}^2(\mathbf{H}^H \mathbf{H})}{\rho} \right) \|\mathbf{z}_q^{k+1} - \mathbf{z}_q^k\|_2^2. \end{aligned}$$

According to Lemma 2, there exists a constant  $C = \min \left\{ \left\{ \frac{\gamma_q(\rho)}{2} \right\}_{q=1}^Q, \left( \frac{\gamma(\rho)}{2} - \frac{\lambda_{\max}^2(\mathbf{H}^H \mathbf{H})}{\rho} \right) \right\}$  such that

$$\begin{aligned} & L_\rho \left( \{\mathbf{x}_q^k, \mathbf{z}_q^k, \mathbf{y}_q^k\}_{q=1}^Q \right) - L_\rho \left( \{\mathbf{x}_q^{k+1}, \mathbf{z}_q^{k+1}, \mathbf{y}_q^{k+1}\}_{q=1}^Q \right) \\ & \geq C \sum_{q=1}^Q \left( \|\mathbf{x}_q^{k+1} - \mathbf{x}_q^k\|_2^2 + \|\mathbf{z}_q^{k+1} - \mathbf{z}_q^k\|_2^2 \right). \end{aligned}$$

Summing both sides of the above inequality from  $k = 1, \dots, K$ , we have

$$\begin{aligned} & L_\rho \left( \{\mathbf{x}_q^1, \mathbf{z}_q^1, \mathbf{y}_q^1\}_{q=1}^Q \right) - L_\rho \left( \{\mathbf{x}_q^{K+1}, \mathbf{z}_q^{K+1}, \mathbf{y}_q^{K+1}\}_{q=1}^Q \right) \\ & \geq \sum_{k=1}^K \left( C \sum_{q=1}^Q \left( \|\mathbf{x}_q^{k+1} - \mathbf{x}_q^k\|_2^2 + \|\mathbf{z}_q^{k+1} - \mathbf{z}_q^k\|_2^2 \right) \right). \end{aligned} \tag{29}$$

Since  $t = \min_k \{k | \sum_{q=1}^Q \left( \|\mathbf{x}_q^{k+1} - \mathbf{x}_q^k\|_2^2 + \|\mathbf{z}_q^{k+1} - \mathbf{z}_q^k\|_2^2 \right) \leq \epsilon\}$ , we can change (29) to

$$L_\rho \left( \{\mathbf{x}_q^1, \mathbf{z}_q^1, \mathbf{y}_q^1\}_{q=1}^Q \right) - L_\rho \left( \{\mathbf{x}_q^{K+1}, \mathbf{z}_q^{K+1}, \mathbf{y}_q^{K+1}\}_{q=1}^Q \right) \geq tC\epsilon. \tag{30}$$

Since we have  $L_\rho\left(\{\mathbf{x}_q^{K+1}, \mathbf{z}_q^{K+1}, \mathbf{y}_q^{K+1}\}_{q=1}^Q\right) \geq L_\rho\left(\{\mathbf{x}_q^*, \mathbf{z}_q^*, \mathbf{y}_q^*\}_{q=1}^Q\right)$ , (30) can be reduced to

$$t \leq \frac{1}{C_\epsilon} \left( L_\rho\left(\{\mathbf{x}_q^1, \mathbf{z}_q^1, \mathbf{y}_q^1\}_{q=1}^Q\right) - L_\rho\left(\{\mathbf{x}_q^*, \mathbf{z}_q^*, \mathbf{y}_q^*\}_{q=1}^Q\right) \right),$$

where  $L_\rho\left(\{\mathbf{x}_q^*\}_{q=1}^Q, \mathbf{z}_q^*, \mathbf{y}_q^*\right) = \ell\left(\mathbf{z}_q^*\right) - \sum_{q=1}^Q \frac{\alpha_q}{2} \|\mathbf{x}_q^*\|_2^2$ , which concludes the proof of Theorem 2. ■

## References

- [1] D. P. Bertsekas, *Convex Optimization Theory*. Belmont, MA, USA: Athena Scientific, 2009.
- [2] S. Boyd and L. Vandenberghe, *Convex Optimization*. Cambridge, U.K.: Cambridge Univ. Press, 2004.
- [3] D. P. Bertsekas, *Nonlinear Programming*, 2nd ed. Belmont, MA, USA: Athena Scientific, 1999.
